# Supplementary material for: Estimating On-road Transportation Carbon Emissions from Open Data of Road Network and Origin-destination Flow Data
Source: arXiv:2402.05153 source file (2024-02-07)
Supplement: Supplementary file 1 [file supplementary.tex]

\begin{table}[t]
\caption {{Summary of Notations.}}
\centering 
\setlength{\tabcolsep}{2mm}
{
\begin{tabular}{c|p{6cm}}
\toprule  
Notation& Description\\
\midrule  
$\mathcal{A}$& Region set.\\
\hline
\multirow{2}*{\makecell[c]{$r$, $c$, $g$}} & The road network level, community level, and region level\\
\hline
\multirow{2}*{\makecell[c]{$\bm{X}^V_r$, $\bm{X}^E_r$, $\bm{X}^B_r$}} & Road intersection attributes, road segment attributes, and between-road attributes \\
\hline
\multirow{2}*{\makecell[c]{$\bm{X}^V_c$, $\bm{X}^E_c$}}& Vertex attributes and edge attributes of the community-level graph  \\
\hline
$\bm{X}^E_g$& Edge attributes of the region-level graph  \\
\hline
\multirow{2}*{\makecell[c]{$\bm{X}^V_{g, \text{intra}}$}} & Region representation learned by intra-region modelling \\
\hline
\multirow{2}*{\makecell[c]{$\bm{X}^V_{g, \text{inter}}$}} & Region representation learned by inter-region modelling \\
\hline
$\bm{X}^V_{g}$ & Region representation by attentional fusion \\
\hline
$\bm{H}$ & Our model \textbf{HANE} \\
\hline
$\bm{H}_{\text{intra}}$ & The intra-region modeling module of $\bm{H}$ \\
\bottomrule 
\end{tabular}
}
\vspace{-3mm}
\label{table:notation}
\end{table}

\begin{algorithm}[h]

    \caption{Learning procedure of \text{HANE}. }
    \begin{algorithmic}[1]
        \STATE \text{Input:} Road network $G=(\bm{V}, \bm{E})$ with road intersection attributes $\bm{X}^V_r$, road segment attributes $\bm{X}^E_r$, and between-road attributes $\bm{X}^B_r$, OD data $\bm{O}$, region set $\mathcal{A}$, on-road carbon emission statistics $\{Y_a|a\in \mathcal{A}\}$.
        \STATE \text{Output:} On-road carbon emission estimates for region $a'$ without observed label.
        \STATE \text{STEP} 1: Pretrain the intra-region module
        \STATE \hspace{0.4cm} Initialize the intra-region module \bm{$H_{\text{intra}}$} and a MLP.
        \STATE \hspace{0.4cm} for $i = 1, 2,..., n_{\text{pretrain}}$ \text{do}
        \STATE \hspace{0.9cm}Sample a minibatch $\mathcal{A}_{\text{batch}} \in \mathcal{A}$ of size $m$;
        \STATE \hspace{0.9cm}Obtain intra-region representation $\bm{X}^{V}_{g, \text{intra}}$ by~\eqref{equ:intra} for $a \in \mathcal{A}_{\text{batch}}$;
        \STATE \hspace{0.9cm}Feed $\bm{X}^{V}_{g, \text{intra}}$ to MLP and get the prediction result $\bm{{\hat{Y}_{a, \text{intra}}}}$ for $a \in \mathcal{A}_{\text{batch}}$;
        \STATE \hspace{0.9cm}Optimize intra-region module $\bm{H_{\text{intra}}}$ with~\eqref{equ:loss}
        \STATE \text{STEP} 2: Train the whole model
        \STATE \hspace{0.4cm} Initialize our prediction model \bm{$H$} and load the pretrained intra-region module $\bm{H_{\text{intra}}}$.
        \STATE \hspace{0.4cm} for $i = 1, 2,..., n_{\text{iter}}$ \text{do}
        \STATE \hspace{0.9cm}Sample a minibatch $\mathcal{A}_{\text{batch}} \in \mathcal{A}$ of size $m$;
        \STATE \hspace{0.9cm}Obtain region representation $\bm{X}^{V}_{g}$ by~\eqref{equ:full} for $a \in \mathcal{A}_{\text{batch}}$;
        \STATE \hspace{0.9cm}Feed $\bm{X}^{V}_{g}$ to MLP and get the prediction result $\bm{{\hat{Y}_{a}}}$ for $a \in \mathcal{A}_{\text{batch}}$;
        \STATE \hspace{0.9cm}Optimize the whole model $\bm{H}$ with loss Equation~\eqref{equ:loss}
    \end{algorithmic} 
    \label{alg}
    \vspace{-1mm}
\end{algorithm}

\begin{itemize}
[leftmargin=5]
    \item \textbf{On-road Carbon Emissions.} On-road carbon emissions refer to the transportation carbon emissions from vehicles moving on roads. For a region, its calculation include the carbon emissions of all vehicle movements inside its administrative boundary. 
    \item \textbf{Road Intersection.} Road intersection refers to the locations where roads cross each other. It represents the connectivity within a road network where people can choose a turning. Therefore, it carries some side features including longitude, latitude, and intersection type (four-way intersections, T-intersections, ...).
    \item\textbf{Road Segment.} Road Segments refer to the standard road unit in the road network system, where each segment connects two adjacent road intersections. The side features of road segments include road class, length, longitude, and latitude.
    \item \textbf{Road Network.} Road network is a combination and organization of road segments and road intersections. Considering the spatiality of road network elements, the road network is often characterized in the graph form $\bm{G} = (\bm{V}, \bm{E})$, where $\bm{V}$ denotes road intersections and $\bm{E}$ denotes road segments.
    \item \textbf{Origin-destination Flow.} Origin-destination flow, short as OD, refers to the number of flows of individuals between specific origins and destinations. In our task, OD indicates the travel demand inside and across regions and is denoted as $\bm{O}$.
    \item \textbf{Community.} Community is a geographic subdivision of regions, typically in a neighborhood form. Residents in a community typically have a more similar lifestyle and share a common travel pattern.
    \item \textbf{Region.} Region refers to an urban geographic or administrative division in our task. It could correspond to a county in the United States, a district in China, or other spatial units according to application scenarios.
\end{itemize}

In east-west divisions, counties of the eastest 17 states are set as the testing set, and the rest counties are set as the training\&validation set; In north-south divisions, counties of the southest 7 states are set as the testing set, and the rest counties are set as the training\&validation set.
